# Supplementary material for: IMAD: IMage-Augmented multi-modal Dialogue
Source: arXiv:2305.10512 source file (2023-12-16)
Supplement: Supplementary file 1 [file appendix_C.tex]

To validate the composed dataset we finetuned two BLIP models from a pre-trained checkpoint. These models consist of ViT-B/16 image encoder and BERT text decoer with 12 layers, 12 attention heads, hidden size of 768, intermediate size of 3072, and GeLU activations \cite{gelu}.
